# Supplementary material for: CodeRAG-Bench: Can Retrieval Augment Code Generation?
Source: arXiv:2406.14497 source file (2025-02-26)
Supplement: Supplementary file 1 [file dataset_documentation.tex]

\section{Appendix: Datasheets for Datasets}

\subsection{Access to \datasetname}
\label{app:a.1:access}
We provide access to view and download all datasets with our additional ground-truth document annotation, as well as all documents from the five retrieval sources at \url{https://huggingface.co/code-rag-bench}. 
For each dataset or retrieval source, the corresponding Croissant metadata can be found via a \texttt{Croissant} tag button on the dataset's page.
All code generation datasets we build upon are permissively licensed. There is no noticeable chance that our data would contain personally identifiable or offensive content.
The codebase for our retrieval-augmented code generation framework can be found at \url{https://github.com/code-rag-bench/code-rag-bench}. 
Overall, all necessary datasets, code, and evaluation procedures are accessible and documented by our main website \url{https://code-rag-bench.github.io/}.

\paragraph{Author Statement}
The authors state that they bear all responsibility in case of violation of rights of the original datasets and retrieval sources. We confirm that the data is released under the CC-BY-SA 4.0 license.
The authors plan to host the dataset and codebase with the above sources on Huggingface and GitHub, and will continue to provide the necessary maintenance to both.

\subsection{Dataset Documentation and Intended Uses}
We provide detailed dataset documentation and explanations for the intended uses, using the datasets for dataset \citep{gebru2021datasheets} framework.

\subsection{Motivation}

\noindent \textbf{For what purpose what the dataset created?} \quad We create \datasetname to provide a unified benchmark for retrieval-augmented code generation, encompassing various code generation tasks and retrieval sources, to facilitate research in this direction.

\noindent \textbf{Who created the dataset and one behalf of which entity?} \quad
Student researchers in Carnegie Mellon University, University of Washington, and University of Southern California created this dataset.

\noindent \textbf{Who funded the creation of the dataset?} \quad
Supervisors of this project, also professors at Carnegie Mellon University funded the creation of this dataset.

\subsection{Composition}

\noindent \textbf{What do the instance that comprise the dataset represent?} \quad
The dataset represents (i) different programming tasks that reflect the job of software developers, and (ii) various reference sources for solving or guiding software programming.

\noindent \textbf{How many instances are there in total?} \quad
Our dataset comprises 9$k$ programming problems and 160$k$ retrieval documents in total.

\noindent \textbf{Does the dataset contain all possible instances or is it a sample of instances from a larger set?} \quad
For code generation datasets, our \datasetname contains all possible instances. For retrieval sources, our \datasetname contains a subset of documents in high quality.

\noindent \textbf{What data does each instance consist of?} \quad
Each example in code generation tasks consists of the problem statement, reference solution, executable test cases, and other necessary metadata specific to individual tasks. 
Each example in retrieval documents contains the textual content and other optional metadata specific to individual sources. All fields in both types are represented by texts.

\noindent \textbf{Is there a label or target associated with each instance} \quad
Each example in code generation tasks is associated with canonical test cases, which serve as the role of labels because model-generated programs need to be executed over and pass all test cases to verify the correctness.
Examples in retrieval documents do not have a label because they are collected for retrieval to augment contexts, instead of end evaluation purposes.

\noindent \textbf{Is any information missing from individual instances?} \quad
No, we did not remove any information collected throughout the process.

\noindent \textbf{Are relationships between individual instances made explicit?} \quad
Yes. We mark examples that are originated from each dataset or each retrieval sources, by putting them into different dataset splits. 

\noindent \textbf{Are there recommended data splits?} \quad
Our \datasetname is built for evaluation purposes and only has the test split, though we do not explicitly split to to `test' since `train' and `validation' sets do not exist.

\noindent \textbf{Are there any errors, sources of noise, or redundancies in the dataset?} \quad
For code generation tasks, we build upon existing high-quality datasets and the authors conduct manual assessments of each dataset. We do not notice any noticeable errors among randomly sampled instances. 
For retrieval sources, we apply several layers to clean the scraped texts, but they may not appear perfectly standard and noises are possible.

\noindent \textbf{Is the dataset self-contained, or does it link to or otherwise rely on external resources?} \quad
Our dataset is self-contained and do not rely on external resources.

\noindent \textbf{Does the dataset contain data that might be considered confidential?} \quad
No, we collect documents from permissively licensed sources.
% \fxcomment{stackexchange and stackoverflow data: cc-by-sa 4.0 licensing; GitHub: GitHub was limited to MIT, BSD, or Apache licenses only}

\noindent \textbf{Does the dataset contain data that, if viewed directly, might be offensive, insulting, threatening, or might otherwise cause anxiety?} \quad
No, we collect programming data, which by default should not involve offensive languages.

\noindent \textbf{Does the dataset identify any subpopulations?} \quad
No, our dataset does not include metadata that are specifically related to any subpopulations (e.g., age, gender).

\noindent \textbf{Is it possible to identify individuals, either directly or indirectly, from the dataset?} \quad
No, our dataset is unlikely to contain user-specific information such as name or other personally identifiable data.% \akari{might be better to just say unlikely, especially given that repoeval and swebench is from existing code bases, they may contains contributors account name or something? }

\noindent \textbf{Does the dataset contain data that might be considered sensitive in any way?} \quad
No.

\subsubsection{Collection Process}
\noindent \textbf{How was the data associated with each instance acquired?} \quad
The data is derived from existing datasets and online resources.

\noindent \textbf{What mechanisms or procedures were used to collect the data?} \quad
We first automatically collect retrieval sources to construct a large-scale document pool. We then iteratively conduct manual verification and content refinement to ensure the data quality.

\noindent \textbf{If the dataset is a sample from a larger set, what was the sampling strategy?} \quad
Only the StackOverflow posts and GitHub repositories are sampled, randomly from the full set.

\noindent \textbf{Who was involved in the data collection process and how were they compensated?} \quad
Graduate student researchers who authored this work were involved in the data collection process. The students were compensated by the authorship of this paper.

\noindent \textbf{Over what timeframe was the data collected?} \quad
March 2024 to May 2024.

\noindent \textbf{Were any ethical review processes conducted?} \quad
No. Because our benchmark does not involve human annotation and is mostly automatic, and the data collected are mainly about programming without raised ethical concerns, we did not find it necessary to conduct ethical reviews.

\subsubsection{Preprocessing/cleaning/labeling}
\noindent \textbf{Was any preprocessing/cleaning/labeling of the data done} \quad
For code generation datasets, we perform manual labeling of the ground-truth documents.
For retrieval documents, we perform necessary cleaning to ensure the quality and clarity of these documents.

\noindent \textbf{Was the “raw” data saved in addition to the preprocessed/cleaned/labeled data?} \quad
Yes, the raw data is accessible through its original sources, which we individually referenced in the main paper.

\noindent \textbf{Is the software that was used to preprocess/clean/label the data available?} \quad
Yes, the software is provided by our codebase.

\subsubsection{Uses}
\noindent \textbf{Has the dataset been used for any tasks already?} \quad
No.

\noindent \textbf{What (other) tasks could the dataset be used for?} \quad
In addition to code generation and retrieval-augmented code generation tasks that we have experimented in this work, our dataset could be potentially extended to other programming tasks or programming document retrieval tasks.

\noindent \textbf{Is there anything about the composition of the dataset or the way it was collected and preprocessed/cleaned/labeled that might impact future uses?} \quad
Our dataset is centered around code generation tasks, but this paradigm could be further extended to other programming-related tasks.

\noindent \textbf{Are there tasks for which the dataset should not be used?} \quad
No.

\subsubsection{Distribution}

\noindent \textbf{Will the dataset be distributed to third parties outside of the entity (e.g., company, institution, organization) on behalf of which the dataset was created?} \quad
No.

\noindent \textbf{How will the dataset will be distributed?} \quad
By Huggingface and GitHub, see the URLs in \S\ref{app:a.1:access}.

\noindent \textbf{When will the dataset be distributed?} \quad
The dataset will be distributed on Jun 6th, 2024.

\noindent \textbf{Will the dataset be distributed under a copyright or other intellectual property (IP) license, and/or under applicable terms of use (ToU)?} \quad
The dataset will be distributed under the Apache 2.0 license.

\noindent \textbf{Have any third parties imposed IP-based or other restrictions on the data associated with the instances?} \quad
No.

\noindent \textbf{Do any export controls or other regulatory restrictions apply to the dataset or to individual instances? } \quad
No.

\subsubsection{Maintainence}

\noindent \textbf{Who will be supporting/hosting/maintaining the dataset?} \quad
The authors of this work will be supporting/hosting/maintaining the dataset. All of the URLs are available at \S\ref{app:a.1:access}.
\noindent \textbf{Is there an erratum?} \quad
No.

\noindent \textbf{Will the dataset be updated?} \quad
No, at least no plans to do so at the submission time.

\noindent \textbf{If the dataset relates to people, are there applicable limits on the retention of the data associated with the instances?} \quad
No, the dataset is not related to people.

\noindent \textbf{Will older versions of the dataset continue to be supported/hosted/maintained?} \quad
We are not planning to update the dataset and will continue to host the current version.

\noindent \textbf{If others want to extend/augment/build on/contribute to the dataset, is there a mechanism for them to do so?} \quad
Yes, we will make our datasets and codebase publicly available, anyone in the community is welcome to contribute or leave comments.
