# Supplementary material for: CodeRAG-Bench: Can Retrieval Augment Code Generation?
Source: arXiv:2406.14497 source file (2025-02-26)
Supplement: Supplementary file 2 [file ablation-studies-deprecated.tex]

% ######### %
\section{Can Top-$k$ documents outperform ground-truth?}
One intriguing phenomenon is that generating with some model-retrieved contexts outperforms generating with ground-truth documents, on Humaneval, MBPP, and DS1000.

\begin{wraptable}{r}{0.56\textwidth}
\vspace{-4mm}
\caption{RACG with top-5 retrieved documents versus with the ground-truth documents.}
\label{tab:top5-vs-gold}
\vspace{1mm}
% \small
    \begin{tabular}{l|ccc}
    \toprule  
    \multicolumn{1}{c|}{\textbf{Method}} & {HumanEval} & {MBPP} & {DS-1000} \\
    \midrule
    {top-5 docs} & {~~97.6} & {92.6} & {35.5} \\
    {top-5 w/o gold} & {~~37.2} & {52.2} & {13.2} \\
    {random 5 docs} & {~~40.9} & {49.2} & {11.8} \\
    {gold + 4 docs} & {100.0} & {99.0} & {13.6} \\
    \bottomrule
    \end{tabular}
\vspace{-1mm}
\end{wraptable}

To investigate the cause of this, we conduct RAG in three alternative settings: (i) \textit{top-5 w/o gold}: remove ground-truth from retrieved documents, then take the top-5 documents from the list, (ii) \textit{random 5 docs}: use 5 random documents sampled from the pool, and (iii) \textit{gold + 4 docs}:  use the ground-truth document plus 4 random sampled documents. We use the OpenAI retrieval results for its superior results, and use StarCoder for generation since it shows the "RAG > Gold" phenomenon on all three datasets.

\zwcomment{add some analysis}



% ######### %
\section{Retrieving Various Amounts of Documents}

\begin{table}[ht]
\caption{(top-2) Performance of retrieval-augmented code generation, with various retrievers and the best performing open- and closed-source generation models.}
\label{tab:rag-top2-docs}
\small
\begin{center}
  \begin{tabular}{l|ccc|cc|cc}
    \toprule
    \multicolumn{1}{c|}{\multirow{2}{*}{\textbf{Method}}} & \multicolumn{3}{c|}{\textbf{General}} & \multicolumn{2}{c|}{\textbf{Open-Domain}} & \multicolumn{2}{c}{\textbf{Repo-Level}} \\
    {} & {HumanEval} & {MBPP} & {LCB} & {DS-1000} & {ODEX} & {RepoEval} & {SWE-bench} \\
    \midrule
    \multicolumn{8}{c}{\textit{w/ DeepseekCoder-7B-instruct}} \\
    \midrule
    \dlrow {None} & {70.1} & {$~~$7.2} & {$~~$0.3} & {41.4} & {39.2} & {33.6} & {} \\
    {BM25} & {97.6} & {33.2} & {} & {35.3} & {35.5} & {} & {} \\
    {GIST-large} & {86.0} & {33.0} & {} & {33.5} & {32.3} & {} & {} \\
    {Voyage, code} & {87.8} & {32.0} & {} & {36.4} & {35.1} & {} & {} \\
    {OpenAI, small} & {97.6} & {34.6} & {} & {34.5} & {35.5} & {} & {} \\
    \hlrow {Gold} & {87.8} & {62.8} & {-} & {43.2} & {41.7} & {48.1} & {} \\
    \midrule
    \multicolumn{8}{c}{\textit{w/ LLaMa3-8B-instruct}} \\
    \midrule
    \dlrow {None} & {57.9} & {$~~$3.6} & {14.3} & {28.9} & {37.4} & {31.2} & {} \\
    {BM25} & {57.3} & {12.6} & {} & {19.8} & {32.6} & {} & {} \\
    {GIST-large} & {45.1} & {9.6} & {} & {23.4} & {31.2} & {} & {} \\
    {Voyage, code} & {53.7} & {9.6} & {} & {21.3} & {32.3} & {} & {} \\
    {OpenAI, small} & {63.4} & {10.2} & {} & {21.4} & {32.3} & {} & {} \\
    \hlrow {Gold} & {65.2} & {29.2} & {-} & {31.1} & {33.7} & {46.3} & {} \\
    \midrule
    \multicolumn{8}{c}{\textit{w/ GPT-3.5-turbo}} \\
    \midrule
    \dlrow {None} & {72.6} & {$~~$1.2} & {28.8} & {43.7} & {41.7} & {} & {} \\
    {BM25} & {} & {} & {} & {} & {} & {} & {} \\
    {GIST-large} & {} & {} & {} & {} & {} & {} & {} \\
    {Voyage, code} & {} & {} & {} & {} & {} & {} & {} \\
    {OpenAI, small} & {} & {} & {} & {} & {} & {} & {} \\
    \hlrow {Gold} & {91.5} & {34.8} & {-} & {42.9} & {40.3} & {} & {} \\
    \bottomrule
  \end{tabular}
\end{center}
\end{table}
